# Supplementary material for: Data-Driven System Level Synthesis
Source: arXiv:2011.10674 source file (2021-03-06)
Supplement: Supplementary file 1 [file fund-lemma-proof.tex]

\section{Proof of Willems' Fundamental Lemma}
\label{sec:fund-lemma-proof}

The proofs in this section are adapted from \cite{van2020willems, de2019persistency}.
We customize the notation to our setting and elaborate
with additional detail where instructive.

\begin{proof}[Lemma~\ref{lem:fund-lemma} (1)]
For notational convenience define
\begin{align*}
    \mcal{H}_{1, L} =
        \begin{bmatrix} \mcal{H}_{1} (z) \\ \mcal{H}_{L} (u) \end{bmatrix},
        \qquad
    \mcal{H}_{1, n + L} =
        \begin{bmatrix} \mcal{H}_{1} (z) \\ \mcal{H}_{n + L} (u) \end{bmatrix}
\end{align*}
and consider a vector
\(\begin{bmatrix} \xi & \eta \end{bmatrix} \in \mbb{R}^{1 \times (n + mL)}\)
in the left-kernel of \(\mcal{H}_{1, L}\):
\begin{align*}
    \begin{bmatrix} \xi & \eta \end{bmatrix}
    \mcal{H}_{1, L}
    =
    \begin{bmatrix} \xi & \eta \end{bmatrix}
    \begin{bmatrix}
        z(0) & z(1) & \cdots & z(T - L) \\
        \hline
        u(0) & u(1) & \cdots & u(T - L) \\
        \vdots & \vdots & \ddots & \vdots \\
        u(L - 1) & u(L) & \cdots & u(T - 1)
    \end{bmatrix}
    = 0_{1 \times (T - L + 1)}
\end{align*}
In other words, this \(\begin{bmatrix} \xi & \eta \end{bmatrix}\)
has the property that on all columns of \(\mcal{H}_{1, L}\),
\begin{align*}
    \xi z(t) + \eta u_{[t, t + L - 1]} = 0 \in \mbb{R},
    \quad 0 \leq t \leq T - L
\end{align*}
The goal of the proof involves showing that
we must have \(\begin{bmatrix} \xi & \eta \end{bmatrix} = 0_{1 \times (n + mL)}\),
and therefore the left-kernel of \(\mcal{H}_{1, L}\) is trivial.
First, a vector in the left-kernel of \(\mcal{H}_{1, n+L}\) is found:
\begin{align*}
    &\begin{bmatrix} \xi & \eta & 0_{1 \times nm}\end{bmatrix}
    \mcal{H}_{1, n + L} \\
    &\quad=
    \begin{bmatrix} \xi & \eta & 0_{1 \times nm}\end{bmatrix}
    \begin{bmatrix}
        z(0) & z(1) & \cdots & z(T - n - L) \\
        \hline
        u(0) & u(1) & \cdots & u(T - n - L) \\
        \vdots & \vdots & \ddots & \vdots \\
        u(L - 1) & u(L) & \cdots & u(T - n - 1) \\
        \hline
        u(L) & u(L + 1) & \cdots & u(T - n) \\
        \vdots & \vdots & \ddots & \vdots \\
        u(n + L - 1) & u(n + L) & \cdots & u(T - 1)
    \end{bmatrix} \\
    &\quad= 0_{1 \times (T - n - L + 1)}
\end{align*}
This \(\begin{bmatrix} \xi & \eta & 0_{1 \times nm} \end{bmatrix}\)
is used to derive additional vectors in the left-kernel of \(\mcal{H}_{1, n+L}\),
from which a new vector in the left-kernel of \(\mcal{H}_{n + L} (u)\) is constructed.
It is then argued via controllability that
\(\begin{bmatrix} \xi & \eta \end{bmatrix} = 0_{1 \times (n + mL)}\) follows.

To derive these additional kernel vectors,
the system dynamics \(z(t + 1) = A z(t) + B u(t)\)
means that the top two block rows of \(\mcal{H}_{1, n + L}\)
are advanced by one step via left-multiplying \(\begin{bmatrix} A & B \end{bmatrix}\):
\begin{align*}
    \begin{bmatrix} A & B \end{bmatrix}
    \begin{bmatrix}
        z(0) & \cdots & z(T - n - L) \\
        u(0) & \cdots & u(T - n - L)
    \end{bmatrix}
    = \begin{bmatrix} z(1) & \cdots & z(T - n - L + 1) \end{bmatrix}
\end{align*}
Consequently, left-multiplying \(\mcal{H}_{1, n+L}\) by
\(\begin{bmatrix} A & B & 0 & \cdots & 0 \end{bmatrix}\)
results in a block-row of shifted states \(\begin{bmatrix} z(1) & z(2) & \cdots & \end{bmatrix}\).
Using this idea another vector in the left-kernel of \(\mcal{H}_{1, n+L}\) is found:
\begin{align*}
    &\begin{bmatrix} \xi A & \xi B & \eta & 0_{1 \times (n - 1)m} \end{bmatrix}
        \mcal{H}_{1, n + L} \\
    &\quad =
        \begin{bmatrix}
            \cdots & \parens{\xi A z(t) + \xi B z(t) + \eta u_{[t + 1, t + L]} + 0} & \cdots
        \end{bmatrix} \\
    &\quad =
        \begin{bmatrix}
            \cdots & \parens{\xi z(t + 1) + \eta u_{[t + 1, t + L]}} & \cdots
        \end{bmatrix} \\
    &\quad =
        \begin{bmatrix}
            \cdots & 0 & \cdots
        \end{bmatrix}
        \tag{Action of \(\begin{bmatrix} \xi & \eta \end{bmatrix}\) on columns of \(\mcal{H}_{1, L}\)} \\
    &\quad = 0_{1 \times (T - n - L + 1)}
\end{align*}
Repeat this argument to derive additional kernel vectors:
\begin{align*}
    \psi_0 &= \begin{bmatrix} \xi & \eta & 0_{1 \times nm} \end{bmatrix} \\
    \psi_1 &= \begin{bmatrix} \xi A & \xi B & \eta & 0_{1 \times (n - 1) m} \end{bmatrix} \\
    \psi_2 &= \begin{bmatrix} \xi A^2 & \xi A B & \xi B & \eta & 0_{1 \times (n - 2) m} \end{bmatrix} \\
     &\vdots & \\
    \psi_n &= \begin{bmatrix} \xi A^n & \xi A^{n - 1} B & \cdots & \xi B & \eta \end{bmatrix}
\end{align*}
such that each \(\psi_i \mcal{H}_{1, n + L} = 0_{1 \times (T - n - L + 1)}\).
However \(\mcal{H}_{n + L} (u)\) has full rank by persistency of excitation,
so the \(n + 1\) vectors \(\psi_0, \psi_1, \ldots, \psi_n\) span at most an \(n\)-dimensional space,
and are therefore linearly dependent.
Given their form, we can conclude that \(\eta = 0_{1 \times mL}\)
since otherwise each \(\psi_{k + 1}\) introduces a new non-zero coordinate
non-existent in \(\psi_0, \ldots, \psi_k\).

Next, by the Cayley-Hamilton theorem there exists
\(\alpha_0, \alpha_1, \ldots, \alpha_n \in \mbb{R}\)
with \(\alpha_n = 1\) and \(\sum_{i = 0}^{n} \alpha_i A^i = 0\).
Then the vector
\begin{align*}
    \sum_{i = 0}^{n} \alpha_i \psi_i
        = \begin{bmatrix}
            0_{1 \times n}
            & \sum_{i = 1}^{n} \alpha_i \xi A^{i - 1} B
            & \sum_{i = 2}^{n} \alpha_i \xi A^{i - 2} B
            & \cdots
            & \alpha_n \xi B
            & 0_{1 \times mL}
        \end{bmatrix}
\end{align*}
is in the left-kernel of \(\mcal{H}_{1, n + L}\) since it is
a linear combination of \(\psi_0, \psi_1, \ldots, \psi_n\).
However this implies that the truncated vector
\begin{align*}
    \begin{bmatrix}
        \sum_{i = 1}^{n} \alpha_i \xi A^{i - 1} B
        & \sum_{i = 2}^{n} \alpha_i \xi A^{i - 2} B
        & \cdots
        & \alpha_n \xi B
        & 0_{1 \times mL}
    \end{bmatrix}
\end{align*}
is in the left-kernel of \(\mcal{H}_{n + L} (u)\),
which is trivial since \(u\) is persistently exciting of order \(n + L\).
In other words, the components of this truncated vector must satisfy
\begin{align*}
    0_{1 \times m} &= \alpha_1 \xi B + \cdots + \alpha_n A^{n - 1} B \\
    0_{1 \times m} &= \alpha_2 \xi B + \cdots + \alpha_n A^{n - 1} B \\
     & \vdots \\
    0_{1 \times m} &= \alpha_{n - 1} \xi B + \alpha_n \xi A B \\
    0_{1 \times m} &= \alpha_n \xi B
\end{align*}
Starting from the last equation: \(\alpha_n = 1\) means that \(\xi B = 0\).
Substituting this into the second-to-last equation yields \(\xi A B = 0\),
and continuing this trend:
\begin{align*}
    \xi B = \xi A B = \cdots = \xi A ^{n - 1} B = 0
\end{align*}
from which controllability of \((A, B)\) implies \(\xi = 0_{1 \times n}\).
From earlier, \(\eta = 0_{1 \times mL}\),
so together it follows that \(\begin{bmatrix} \xi & \eta \end{bmatrix}\) is zero.
As this was an arbitrary vector in the left-kernel of \(\mcal{H}_{1, L}\),
conclude that \(\mcal{H}_{1, L}\) has a trivial left-kernel.
\end{proof}

%%%%%%%%%%%%%%%%%%%%%%%%%%%%%%%%%%%%%%%%%%%%%%%%%%%%%%%%%%%%%%%%%%%%%%%%%%%%%%%%%%%%%%%%%%

\begin{proof}[Lemma~\ref{lem:fund-lemma} (2)]
Assuming that
\begin{align*}
    \rank
    \begin{bmatrix} \mcal{H}_{1} (z) \\ \mcal{H}_{L} (u) \end{bmatrix}
    = n + mL
\end{align*}
implies the existence of a \(g \in \mbb{R}^{T - L + 1}\) such that
\begin{align*}
    \begin{bmatrix}
        \bar{x}(0) \\ \bar{u}_{[0,  L - 1]}
    \end{bmatrix}
    = \begin{bmatrix} \mcal{H}_{1} (z_{[0, T - L]}) \\ \mcal{H}_{L} (u_{[0, T - 1]}) \end{bmatrix} g
\end{align*}
for all desired initial states \(\bar{x}(0)\) and control trajectory \(\bar{u}_{[0, L - 1]}\).
Substituting this into the following
relation yields the desired output and control trajectory
as a parameter of \(g\):
\begin{align*}
    \begin{bmatrix} \bar{x}_{[0, L - 1]} \\ \bar{u}_{[0, L - 1]} \end{bmatrix}
    = \begin{bmatrix} \begin{array}{c|c}
        \mcal{O}_L (A) & \mcal{T}_{L} (B) \\
        \hline
        0_{nL \times n} & I_{mL}
        \end{array}\end{bmatrix}
      \begin{bmatrix} \bar{x}(0) \\ \bar{u}_{[0, L - 1]} \end{bmatrix}
    = \begin{bmatrix} \begin{array}{c|c}
        \mcal{O}_L (A) & \mcal{T}_{L} (B) \\
        \hline
        0_{nL \times n} & I_{mL}
        \end{array}\end{bmatrix}
        \begin{bmatrix}
            \mcal{H}_{1} (z) \\ \mcal{H}_{L} (u)
        \end{bmatrix}
        g
\end{align*}
\end{proof}
