# Supplementary material for: Data-Driven System Level Synthesis
Source: arXiv:2011.10674 source file (2021-03-06)
Supplement: Supplementary file 2 [file intermediate-results.tex]

\section{Proofs and Intermediate Results}
