# Supplementary material for: Data-Driven System Level Synthesis
Source: arXiv:2011.10674 source file (2021-03-06)
Supplement: Supplementary file 3 [file appendix.tex]

\appendix
\section{Proofs and Intermediate Results}
